# Supplementary material for: RAG-Modulo: Solving Sequential Tasks using Experience, Critics, and Language Models
Source: arXiv:2409.12294 source file (2024-09-18)
Supplement: Supplementary file 1 [file appendix.tex]

\newpage
\section*{APPENDIX}
